# Supplementary material for: Efficient and High-Quality Seeded Graph Matching: Employing High Order Structural Information
Source: arXiv:1810.11152 source file (2018-10-26)
Supplement: Supplementary file 1 [file Full_7appendix.tex]

%\pagebreak
%\nobalance
\begin{appendix}
\addcontentsline{toc}{section}{Appendix}

\subsection{Proof}  \label{7proof}
\subsubsection{Proof of Lemma~\ref{lemma1}} \label{7lemma1}
%\textbf{1. Proof of Lemma~\ref{lemma1}.}
\begin{proof}%[\unskip\nopunct]
The effectiveness of postponing strategy is analysed on the $G(n,p;p_n,p_e)$ random graph model. Assume $G(V, E)$ is the graph generated from Erd\"os-Renyi random graph model $G(n,p)$,
% i.e., $|V|=n$ and $(i,j)\in E$ with probability $p$ for any $i,j\in V$;
and $G_1(V_1, E_1)$ and $G_2(V_2, E_2)$ are two subgraphs sampled from $G(V, E)$.
Assume vertex  $s, v\in V_1$, $s',u\in V_2$, and $[s,s']$ is a matched seed, we define $\mathtt{Score_s}(v,u)$ by
\[
    \mathtt{Score}_s(v,u)=
\begin{cases}
    1 & seed\ pair\ [s,s']\ percolates\ $1$ \ mark \ to \\
                   & [v,u] \ after \ one \ iteration,\\
    0              & \text{otherwise.}
\end{cases}
\]
Thus $\mathtt{Score}_s(v,u)=1$ only if $(s,v)\in E_1$ and $(s',u)\in E_2$.
If both $[s,s']$ and $[v,u]$ are correct matches (in $G$), then the probability that $(s,v)\in E$ and $(s',u)\in E$ is $p$; otherwise, the probability is $p^2$. Thus, we have the following equation:
\[
    Pr(\mathtt{Score}_s(v,u)=1)=
\begin{cases}
    p\cdot p_e^2 &  pair\ [s,s']\ and \ [v,u]  \\
                &    are\ correct\ matches, \\
    p^2 \cdot p_e^2   & \text{otherwise,}
\end{cases}
\]
%which represents the probability that $[v,u]$ obtains $1$ mark from the pair $[s,s']$.
Then we consider the precision and recall of matching in each iteration; we assume there are currently $n_c$ correct matches and $n_w$ wrong matches in the matched set $M$.

Firstly, we will prove that the postponing strategy improve the precision by decreasing the probability that a wrong pair is matched in each iteration.
Assume $[v,u']$ and $[v',u]$ are correct matches on $G$ and $[v,u]$ is a wrong match.
We say a pair $[i,j]$ exists in matching if $i\in V_1$ and $j\in V_2$.
There are three cases considering the existence of $[v,u']$ and $[v',u]$:
(1) Neither $[v,u']$ nor $[v',u]$ exists with probability $(1-p_n^2)^2$;
(2) One of $[v,u']$ and $[v',u]$ exists with probability $2\cdot (1-p_n^2)\cdot p_n^2$;
(3) Both $[v,u']$ and $[v',u]$ exist with probability $p_n^4$.
In case (1), the wrong pair $[v,u]$ can be directly matched if $[v,u]$ obtains at least two marks (the probability that any adversary pair of $[v,u]$ receives at least two marks is negligible), the probability of which is $p^4p_e^4(n_c+n_w)^2$.
%In case (2), w.l.o.g., we assume $[v,u']$ exists, the probability that $[v,u]$ has at least $2$ scores and the score of $[v,u]$ is greater than that  of $[v,u']$ is represented by
In case (2), w.l.o.g., we assume $[v,u']$ exists, the probability that $\mathtt{Score}_S(v,u)\ge 2$ and $\mathtt{Score}_S(v,u)-\mathtt{Score}_S(v,u')\ge 1$ is
%\[
%\begin{split}
%    & Pr\Basics[\Big]{\sum_{[s_1,s_2]}{(X_{s_1, s_2,i,j})}\ge 2, \sum_{[s_1,s_2]}{(X_{s_1, s_2,i,j}-X_{s_1,s_2, i, j_1})}\ge 1} \\
%    & = Pr\Basics[\Big]{\sum_{[s_1,s_2]}{(X_{s_1, s_2,i,j})}\ge 2}  \\
%                                                                                            &  \times   Pr\Basics[\Big]{\sum_{[s_1,s_2]}{(X_{s_1, s_2,i,j}-X_{s_1,s_2, i, j_1})}\ge 1 \given  \sum_{[s_1,s_2]}{(X_{s_1, s_2,i,j})}\ge 2}
%   % & = Pr[\Basics[\Big]{\sum_{[s_1,s_2]}{p \cdot \Basics[\Big]{X_{s_1, s_2,i,j}-X_{s_1,s_2, i, j_1}  \given [s_1,i]\in E_1}}\ge 1 \given \sum_{[s_1,s_2]}{(X_{s_1, s_2,i,j})}\ge 2}]
%\end{split}
%\]
%As $np\to c_1>1$, we have $\frac{1}{p^2}\gg n$, and the probability above can be
approximated by
$p^4p_e^4(n_c^2(1-p_e^4)+n_c n_w(1-p^2p_e^4)+n_c n_w+n_w^2)=p^4p_e^4(n_c+n_w)^2-p^4p_e^4n_c^2p_e^4$ (because $G(n,p)$ model assumes $np$ is a constant greater than $1$, we have $\frac{1}{p^2}\gg n$, and some items are pruned).
In case (3), the probability that $\mathtt{Score}_S(v,u)\ge 2$ and $\mathtt{Score}_S(v,u)-\mathtt{Score}_S(v,u')\ge 1$ and $\mathtt{Score}_S(v,u)- \mathtt{Score}_S(v',u)\ge 1$ should be approximated by  $p^4p_e^4(n_c^2(1-p_e^4)^2+2n_c n_w(1-p^2p_e^4)+n_w^2)$.
By summarizing all three cases, the probability that a wrong pair $[v,u]$ is matched in each iteration under the postponing strategy is  $(n_c+n_w)^2 p^4 p_e^4 - n_c^2 p^4 p_e^4 (2p_e^4-p_e^8+ 2 p_n^2 p_e^4 - 2p_n^4 p_e^4)$.

Secondly, we will show the postponing strategy will not affect the recall of matching, because a correct pair that is matched without the postponing strategy is still matched w.h.p. under the new rule.
For a correct pair $[v,u]$, it receives at least $2$ marks at a percolation with probability $n_c^2 p^2 p_e^4$
(which dominates the probability of receiving marks from the wrong seeds when $n_c\gg n_wp$). Because $[v,u]$ has at most $2n-1$ adversary pairs, the probability that $\mathtt{Score}_S(v,u)\ge 2$ and $\mathtt{Score}_S(v',u')\le 1$
for all $[v',u']$ in $\{v\}\times V_2$ and $V_1 \times \{u\}$ excluding $[v,u]$ (consequently, $[v,u]$ is matched) is approximated by $n_c^2 p^2 p_e^4 (1-2np^2)$, which is close to $n_c^2 p^2 p_e^4$ since $\frac{1}{p^2}\gg n$.
\end{proof}

\subsection{Global alignment on random graph}  \label{7alignment}

In Erd\"os-Renyi random graph, assume $np\ge c_1>1$ where $c_1$ is a constant,
then w.h.p. the graph will have a unique giant component containing a positive fraction of the vertices.
In the following analysis, we consider the matching on vertices in this giant component only.
%as it is rather meaningless and difficult to do matching on the small components (each with no more than $O(\log(n))$ vertices).

Firstly, we define a new kind of \emph{signature vector} $D(v)$ for vertex $v$ based on the shortest path distances, which is a simplified version of $R(v)$ based on PPR values.
Let $d(s,v)$ be the shortest path distance from $s$ to $v$, and $D(v)=\{d(s_1,v), d(s_2,v), d(s_3,v), \cdots\}$.
Then we can show that any vertex $v$ in random graph can be uniquely distinguished by $D(v)$ w.h.p. with only a limited number of seeds.

\begin{lemma}\label{lemma2}
In Erd\"os-Renyi random graph, assume $c$ is a large constant, when $\log(n^3)/\log(\frac{cnp}{cnp-1})$ seeds are provided, then $\forall v,u\in V$, $D(v)\ne D(u)$ with probability $1-\frac{1}{n}$.
\end{lemma}

\begin{proof}
Denote $Y^r_v$ the set of nodes the distance from which to node $v$ is $r$.
%and $Y^{\le r}_{i}=\bigcup^{r}_{c=1} Y^{c}_{i}$ the set of nodes the distance from which to node $i$ is no greater than $r$.
Given two randomly picked node $v,u\in V$, then the probability that the distance from a random seed $s_k$ to node $v$ is the same as the distance from $s_k$ to node $u$ is $\sum^{\infty}_{r=1}Pr(s_k\in Y^r_v\ and\ s_k\in Y^r_u) = Pr((\sum^{\infty}_{r=1}{|Y^r_v \cap Y^r_u|})/n)$. Firstly we will prove $1-Pr((\sum^{\infty}_{r=1}{|Y^r_v \cap Y^r_u|})/n)= O(\frac{1}{np})$.

There is no existing work in the literature of random graph that approximates $|Y^r_v|$ well with strong guarantee for $r=1,2,3,\cdots$. However, according to Chernoff bound, $|Y^{r+1}_v|\le c\cdot np|Y^{r}_v|$ holds for $r=1,2,3,\cdots$ with high probability with a large constant $c$ (the probability is $1-\exp(-O(n))$ when $|Y^{r+1}_v|\to O(n)$), thus w.h.p. $|Y^r_v|\le \frac{cnp-1}{cnp}n$ for $r=1,2,3,\cdots$.

Note that $\sum^{\infty}_{r=1}Pr(s_k\in Y^r_v\ and\ s_k\in Y^r_u)=\sum^{\infty}_{r=1}Pr(s_k\in Y^r_v)\cdot Pr(s_k\in Y^r_u \given s_k\in Y^r_v)$. And $s_k\in Y^r_v$ and $s_k\in Y^k_u$ have dependency. However, we can show that the effect of dependency is limited and can be neglected.

Denote $\mathcal{P}_{v,s_k}$ the shortest paths from $v$ to $s_k$, $\mathcal{P}_{u,s_k}$ the shortest paths from $u$ to $s_k$, then a path $w_1\in \mathcal{P}_{v,s_k}$ shares no edge with a path $w_2\in \mathcal{P}_{u,s_k}$ with a high probability $1-O(\frac{1}{np})$ (proof omitted). % and $w_1$ shares more than $1$ edge with $w_2$ with probability $o(\frac{1}{n^2p^2})$.
We simply consider the case where $w_1\in\mathcal{P}_{v,s_k}$ and $w_2\in\mathcal{P}_{u,s_k}$ share no edges. Since $s_k$ is randomly selected from $V$, $Pr(s_k\in Y^r_v)=|Y^r_v|/n$. Thus we have
\[
\begin{split}
& 1-\sum^{\infty}_{r=1}Pr(s_k\in Y^r_v\ and\ s_k\in Y^r_u) \\
& \ge (1-O(\frac{1}{np}))(1-\sum^{\infty}_{r=1}Pr(s_k\in Y^r_v)\cdot Pr(s_k\in Y^r_u)) \\
& \ge (1-O(\frac{1}{np}))(1-(\frac{cnp-1}{cnp})^2-(\frac{1}{cnp})^2) \\
& \ge (1-O(\frac{1}{np}))\frac{1}{cnp},
\end{split}
\]
which represents the lower bound of the probability that the distance from a random seed $s_k$ to node $v$ is the different from the distance from $s_k$ to node $u$. Then we consider the whole seed set instead of a single seed.
Recall that $D_{v}=\{d(s_1,v), d(s_2,v), d(s_3,v), \cdots\}$ is vector of shortest path distances from the seeds to node $v$. Assume each seed $s_k\in S$ is randomly selected from $V$ independently. Apparently, when $|S|\ge \frac{\log(n^3)}{\log(\frac{cnp}{cnp-1})}$, then with probability $1-(1-(1-\frac{1}{cnp})^{|S|})^{n^3} \approx 1-\frac{1}{n}$, it satisfies $D_{v}\ne D_{j}$ for $\forall v,u\in V$.
\end{proof}

When $cnp\to c_2>2$ (where $c_2$ is a constant), each vertex in Erd\"os-Renyi random graph can be uniquely distinguished by $D(v)$ with a seed set of size $|S|\ge O(\log(n))$.

% Build the connection between the PPR labelling and shortest path distance labelling.
Note the $R(v)$ is much complicated than $D(v)$:
(1) the random walk in PPR is decayed by both $\alpha$ and $1/N(u)$ for each $u$ on the random walk path;
(2) $\pi(s,v)$ also demonstrates the local structural information of $v$, as shown in analysis above;
(3) $\pi(s,v)$ considers multiple random walk paths from $s$ to $v$, rather than the shortest paths only.
We stress the $R(v)$ practically has much greater power in distinguishing the vertices than $D(v)$ which is designed for the purpose of analysis.
%while we use the above simplified version in analysis to avoid much dependency.
% how to PPR.

\subsection{Time complexity of EWS}  \label{7EWS}
We provide the time analysis of EWS~\cite{kazemi2015growing}. The details of EWS is presented in Section~\ref{sec1}.
We assume both graphs in matching contain $O(|V|)$ vertices and $O(|E|)$ edges for simplicity.
Because EWS adds $1$ marks to the neighboring pairs of a matched pair, the percolation and the matching score computation are conducted simultaneously and take the same complexity.
%then we simply consider the complexity of percolation.
Denote $C'$ the set of candidate pairs considered by EWS (receive at least $1$ mark), then the time complexity of percolation is bounded by $O(|C'|)$.
%Further, since each candidate pair $[v,u]$ receives at most $\min(|N(v)|,|N(u)|)$ marks, the total number of percolation (add $1$ mark) is bounded by $O(\frac{|C'||E|}{|V|})$.
We then bound $|C'|$.
Denote $|E^{(2)}|$ the number of non-zero entries in the matrix $(A+A^2)$, where $A$ is the adjacency matrix representing graph $G$ (defined in Section~\ref{21notation}).
Then the summed number of $1$-hop neighbors and $2$-hop neighbors of a vertex is on average $\frac{|E^{(2)}|}{|V|}$.
Thus, each matched pair can produce $O(\frac{|E^{(2)}|^2}{|V|^2})$ candidate pairs (a \emph{noisy pair} also percolates). Because there are at most $|V|$ matched pairs, $|C'|$ is bounded by $O(\frac{|E^{(2)}|^2}{|V|})$.
In conclusion, the time complexity of EWS is $O(\frac{|E^{(2)}|^2}{|V|})$.

%\subsection{Effect of exploiting order-2 structural information.}  \label{7order2}
%
%% order-2 signature.
%% let $s=p_n, t=p_e$
%% If $[s,s']$ and $[v,v]$ are correct matches:
%% order-1: Pr((s,v)\in E) = p.   W ~ B(1,p),  Z ~ B(W, t)   Pr(s->v)=pt^2
%% order-2:
%% # of neighbors of $s$ on G is X ~B(n, p).
%% # of 2-hops from s to v on G is  Y~ B(X, p)
%% # of 2-hops from s to any vertices is Z ~ B(X, p)
%
%% # of 2-hops from s to v (or s' to v) is Y_1 ~ B(Y, st^2)  (Y_2 ~ B(Y, st^2))
%% # of 2-hops from s to any vertices is Z_1 ~ B(Z, st^2)
%
%% X is the number of trials, ~ np in expectation.  (similar to 1-hop analysis, except for an additional factor of st, correct pt^2 to ps^2t^4, and wrong p^2t^2 to p^2s^2t^4).
%% but the results of all trials stacks
%% we can simply consider 1 (2-hop) path from s to v, and 1 path from s' to v.  (the probability of a multi-path is decreased by at least pst^2)
%% For a correct pair: Pr for [v,v] get score 1 from [s,s']  is Ys^2t^4 = Xps^2t^4,  (additional, Pr for score=1/2 is  3X^2p^2s^3t^6)
%
%% distinguish adversary pairs or irrelevant pairs?  seems not necessary.. because size different by n, and Y ~ Z.
%% For a wrong adversary pair: Pr for [v',u'] get score 1 from [s,s'] is  Zp Zp s^2t^4 = X^2p^2s^2t^4.
%
%% consider pi(s,v) is 1-hop + lambda*2-hop.  If W=1, Y=1 with pr= np^3, small pr; ...  consider W=1,Y=0 and W=0, Y=1
%%so for correct pair, pr(sc=1) = pt^2 + X ps^2t^4.
%% for wrong pair, similar, pr(sc=1) = p^2t^2 + X^2p^2s^2t^4
%
%We will show that
%exploiting the order-2 structural information
\end{appendix}
