# Supplementary material for: Efficient and High-Quality Seeded Graph Matching: Employing High Order Structural Information
Source: arXiv:1810.11152 source file (2018-10-26)
Supplement: Supplementary file 2 [file 7appendix.tex]

%\pagebreak
%\nobalance
\begin{appendix}
\addcontentsline{toc}{section}{Appendix}

\subsection{Proof}  \label{7proof}
\subsubsection{Proof of Lemma~\ref{lemma1}} \label{7lemma1}
%\textbf{1. Proof of Lemma~\ref{lemma1}.}
\begin{proof}%[\unskip\nopunct]
The effectiveness of postponing strategy is analysed on the $G(n,p;p_n,p_e)$ random graph model. Assume $G(V, E)$ is the graph generated from Erd\"os-Renyi random graph model $G(n,p)$,
% i.e., $|V|=n$ and $(i,j)\in E$ with probability $p$ for any $i,j\in V$;
and $G_1(V_1, E_1)$ and $G_2(V_2, E_2)$ are two subgraphs sampled from $G(V, E)$.
Assume vertex  $s, v\in V_1$, $s',u\in V_2$, and $[s,s']$ is a matched seed, we define $\mathtt{Score_s}(v,u)$ by
\[
    \mathtt{Score}_s(v,u)=
\begin{cases}
    1 & seed\ pair\ [s,s']\ percolates\ $1$ \ mark \ to \\
                   & [v,u] \ after \ one \ iteration,\\
    0              & \text{otherwise.}
\end{cases}
\]
Thus $\mathtt{Score}_s(v,u)=1$ only if $(s,v)\in E_1$ and $(s',u)\in E_2$.
If both $[s,s']$ and $[v,u]$ are correct matches (in $G$), then the probability that $(s,v)\in E$ and $(s',u)\in E$ is $p$; otherwise, the probability is $p^2$. Thus, we have the following equation:
\[
    Pr(\mathtt{Score}_s(v,u)=1)=
\begin{cases}
    p\cdot p_e^2 &  pair\ [s,s']\ and \ [v,u]  \\
                &    are\ correct\ matches, \\
    p^2 \cdot p_e^2   & \text{otherwise,}
\end{cases}
\]
%which represents the probability that $[v,u]$ obtains $1$ mark from the pair $[s,s']$.
Then we consider the precision and recall of matching in each iteration; we assume there are currently $n_c$ correct matches and $n_w$ wrong matches in the matched set $M$.

Firstly, we will prove that the postponing strategy improve the precision by decreasing the probability that a wrong pair is matched in each iteration.
Assume $[v,u']$ and $[v',u]$ are correct matches on $G$ and $[v,u]$ is a wrong match.
We say a pair $[i,j]$ exists in matching if $i\in V_1$ and $j\in V_2$.
There are three cases considering the existence of $[v,u']$ and $[v',u]$:
(1) Neither $[v,u']$ nor $[v',u]$ exists with probability $(1-p_n^2)^2$;
(2) One of $[v,u']$ and $[v',u]$ exists with probability $2\cdot (1-p_n^2)\cdot p_n^2$;
(3) Both $[v,u']$ and $[v',u]$ exist with probability $p_n^4$.
In case (1), the wrong pair $[v,u]$ can be directly matched if $[v,u]$ obtains at least two marks (the probability that any adversary pair of $[v,u]$ receives at least two marks is negligible), the probability of which is $p^4p_e^4(n_c+n_w)^2$.
%In case (2), w.l.o.g., we assume $[v,u']$ exists, the probability that $[v,u]$ has at least $2$ scores and the score of $[v,u]$ is greater than that  of $[v,u']$ is represented by
In case (2), w.l.o.g., we assume $[v,u']$ exists, the probability that $\mathtt{Score}_S(v,u)\ge 2$ and $\mathtt{Score}_S(v,u)-\mathtt{Score}_S(v,u')\ge 1$ is
%\[
%\begin{split}
%    & Pr\Basics[\Big]{\sum_{[s_1,s_2]}{(X_{s_1, s_2,i,j})}\ge 2, \sum_{[s_1,s_2]}{(X_{s_1, s_2,i,j}-X_{s_1,s_2, i, j_1})}\ge 1} \\
%    & = Pr\Basics[\Big]{\sum_{[s_1,s_2]}{(X_{s_1, s_2,i,j})}\ge 2}  \\
%                                                                                            &  \times   Pr\Basics[\Big]{\sum_{[s_1,s_2]}{(X_{s_1, s_2,i,j}-X_{s_1,s_2, i, j_1})}\ge 1 \given  \sum_{[s_1,s_2]}{(X_{s_1, s_2,i,j})}\ge 2}
%   % & = Pr[\Basics[\Big]{\sum_{[s_1,s_2]}{p \cdot \Basics[\Big]{X_{s_1, s_2,i,j}-X_{s_1,s_2, i, j_1}  \given [s_1,i]\in E_1}}\ge 1 \given \sum_{[s_1,s_2]}{(X_{s_1, s_2,i,j})}\ge 2}]
%\end{split}
%\]
%As $np\to c_1>1$, we have $\frac{1}{p^2}\gg n$, and the probability above can be
approximated by
$p^4p_e^4(n_c^2(1-p_e^4)+n_c n_w(1-p^2p_e^4)+n_c n_w+n_w^2)=p^4p_e^4(n_c+n_w)^2-p^4p_e^4n_c^2p_e^4$ (because $G(n,p)$ model assumes $np$ is a constant greater than $1$, we have $\frac{1}{p^2}\gg n$, and some items are pruned).
In case (3), the probability that $\mathtt{Score}_S(v,u)\ge 2$ and $\mathtt{Score}_S(v,u)-\mathtt{Score}_S(v,u')\ge 1$ and $\mathtt{Score}_S(v,u)- \mathtt{Score}_S(v',u)\ge 1$ should be approximated by  $p^4p_e^4(n_c^2(1-p_e^4)^2+2n_c n_w(1-p^2p_e^4)+n_w^2)$.
By summarizing all three cases, the probability that a wrong pair $[v,u]$ is matched in each iteration under the postponing strategy is  $(n_c+n_w)^2 p^4 p_e^4 - n_c^2 p^4 p_e^4 (2p_e^4-p_e^8+ 2 p_n^2 p_e^4 - 2p_n^4 p_e^4)$.

Secondly, we will show the postponing strategy will not affect the recall of matching, because a correct pair that is matched without the postponing strategy is still matched w.h.p. under the new rule.
For a correct pair $[v,u]$, it receives at least $2$ marks at a percolation with probability $n_c^2 p^2 p_e^4$
(which dominates the probability of receiving marks from the wrong seeds when $n_c\gg n_wp$). Because $[v,u]$ has at most $2n-1$ adversary pairs, the probability that $\mathtt{Score}_S(v,u)\ge 2$ and $\mathtt{Score}_S(v',u')\le 1$
for all $[v',u']$ in $\{v\}\times V_2$ and $V_1 \times \{u\}$ excluding $[v,u]$ (consequently, $[v,u]$ is matched) is approximated by $n_c^2 p^2 p_e^4 (1-2np^2)$, which is close to $n_c^2 p^2 p_e^4$ since $\frac{1}{p^2}\gg n$.
\end{proof}
